# Supplementary material for: Modeling Multiple Normal Action Representations for Error Detection in Procedural Tasks
Source: arXiv:2503.22405 source file (2025-04-02)

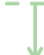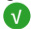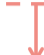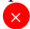

Supplement: Supplementary file 1 [file normal_and_error_cropped.pdf]
